# Supplementary material for: A Benchmark Comparison of Learned Control Policies for Agile Quadrotor Flight
Source: arXiv:2202.10796 source file (2022-02-22)
Supplement: Supplementary file 1 [file supplementary.tex]

\section*{Supplementary Material}\label{sec:supplementary}

In the supplementary material we provide implementation details of our quadrotor simulation, training hyperparameters, reference trajectories and the MPC baselines. Additionally, we show a set of additional ablation studies regarding the choice of low level controller, the history length $H$, and the reference length $R$.

\subsection{Training Details}
The policies are trained in a simulated quadrotor environment implemented using TensorFlow Agents. 
The nominal quadrotor parameters such as mass and inertia are identified from the real platform and are summarized in Table~\ref{tab:phys_params} together with the amount of randomization applied at training time. 

\begin{table}[h]
    \centering
    \begin{tabularx}{0.8\linewidth}{X|ccc}
    Parameter & Nominal Value & Randomization\\
    \midrule
    Mass [\SI{}{\kilogram}] & 0.768 & $\pm 30\%$ \\
    Inertia [\SI{}{\kilogram\meter\squared}] & [2.5e-3, 2.1e-3, 4.3e-3] & $\pm 30\%$\\
    Gravity [\SI{}{\meter\per\second\squared}] & [0.0, 0.0, -9.81] & $\pm 0.4$\\
    $k_{vx}$ [\SI{}{\newton\second\per\meter}] & 0.3 & $\pm 0.3$\\
    $k_{vy}$ [\SI{}{\newton\second\per\meter}] & 0.3 & $\pm 0.3$\\
    $k_{vz}$ [\SI{}{\newton\second\per\meter}] & 0.15 & $\pm 0.15$\\
    $c_l$ [\SI{}{\newton\per\radian\per\second}] & 1.563e-6 & $\pm 0.0$\\
    $c_d$ [\SI{}{\newton\meter\per\radian\per\second}] & 1.909e-8 & $\pm 0.0$\\
    \end{tabularx}
    \vspace{3pt}
    \caption{Physical parameters of the simulation. At the start of each rollout, the parameters are sampled from a uniform distribution around the nominal values with the randomization specified above.}
    \label{tab:phys_params}
\end{table}

All policies are trained using PPO using the hyperparameters specified in Table~\ref{tab:ppo_params}.
\begin{table}[h]
    \centering
    \begin{tabularx}{0.5\linewidth}{X|c}
    Hyperparameter & Value\\
    \midrule
    $\gamma$ (discount factor)  & 0.98\\
    Actor learning rate & 3e-4 \\
    Critic learning rate & 3e-4 \\
    Entropy regularization & 1e-2 \\
    $\varepsilon$ (importance ratio clipping) & 0.2
    \end{tabularx}
    \vspace{3pt}
    \caption{Training hyperparameters.}
    \label{tab:ppo_params}
\end{table}

\mypara{Reward Components} 
The episode is terminated when the quadrotor crashes (i.e. $p_z \leq 0.0$) with a reward of $r_\text{crash} = -500$. 
During trajectory tracking, the agent receives at each timestep a reward that penalizes tracking error and deviation from the reference action as laid out in Eq.~\eqref{eq:reward}.
The matrices $\bm{Q}$ and $\bm{R}$ have nonzero elements only on the diagonal. 
Specifically, we use ${\bm{Q} = \text{diag} \lbrace 0.1 \cdot \mathbf{1}_{3\times1},0.02 \cdot \mathbf{1}_{9\times1},0.002 \cdot \mathbf{1}_{3\times1},0.01 \cdot \mathbf{1}_{3\times1}  \rbrace}$ and ${\bm{R} = \text{diag} \lbrace 0.001 \cdot \mathbf{1}_{4\times1}\rbrace}$.

\rev{
\subsection{MPC Baselines}
This section gives a brief overview of the MPC baselines implemented in this work.
MPC stabilizes a system subject to its dynamics $\dot{\bm{x}} = \bm{f}_{dyn}(\bm{x}, \bm{u})$ along a reference ${\bm{x}^*(t), \bm{u}^*(t)}$, where $\bm{f}_{dyn}$ is represented by Eq.~\eqref{eq:3d_quad_dynamics}, omitting the dynamics of the motors.
In each control update, MPC minimizes a cost $\mathcal{L}(\bm{x}, \bm{u})$ as in:
\begin{align}
\min_{\bm{u}} &\int \mathcal{L}(\bm{x}, \bm{u}) \\
\text{subject to } \quad 
\quad \dot{\bm{x}} &= \bm{f}_{dyn}(\bm{x}, \bm{u}) \nonumber \\
\bm{x}(t_0) &= \bm{x}_{init} \nonumber \\
\bm{h}(\bm{x}, \bm{u}) &\leq 0 \nonumber
\end{align}
where $\bm{x}_0$ denotes the initial condition, $\bm{f}_{dyn}$ implements the system dynamics as equality constraints, and $\bm{h}$ represents inequality constraints, such as input limitations.\\
For our application, and as most commonly done, we specify the cost to be of quadratic form $\mathcal{L}(\bm{x}, \bm{u}) = \| \bm{x} - \bm{x}^*  \|^2_Q + \| \bm{u} - \bm{u}^* \|^2_R$ and discretize the system into $N$ steps over time horizon $T$ of size $dt=T/N$.
We account for input limitations by constraining $0 \leq \bm{u} \leq u_{max}$.
\begin{align}
\min_{u} \bm{x}_N^\intercal Q \bm{x}_N + &\sum_{k=0}^N \bm{x}_k^\intercal Q \bm{x}_k + \bm{u}_k^\intercal R \bm{u}_k \\
\text{subject to} \quad
\bm{x}_{k+1} &= \bm{f}_{RK4}(\bm{x}_k, \bm{u}_k, \delta t) \nonumber \\
\bm{x}_0 &= \bm{x}_{init} \nonumber \\
u_{min} & \leq \bm{u}_k \leq u_{max} \nonumber 
\end{align}
where $\bm{f}_{RK4}$ represents the discretized dynamics $\bm{f}_{dyn}$ using a 4th-order Runge-Kutta scheme.
To solve this quadratic optimization problem, we construct it using a multiple shooting scheme and solve it through a sequential quadratic program (SQP) executed in a real-time iteration scheme.
All implementations are done using ACADO~\cite{houska2011acado}.
Both MPC baselines in this work (MPC-SRT and MPC-CTBR) use the same formulation. %
While MPC-SRT forwards the predicted single rotor thrusts to the motors, 
in case of MPC-CTBR the bodyrates and collective thrust from the first predicted state are used as setpoints for the low level controller. 
}

\subsection{Ablation Studies}
We ablate the performance of our trained policies to investigate the impact of the history length $H$ and the reference length $R$, and analyze the sensitivity to the tuning of the low-level controller.

\rev{
\mypara{Sensitivity to Low-Level Controller}
We investigate the sensitivity of the CTBR control policies to the tuning of the underlying low-level controller. 
The low-level controller consists of a PD-controller that tracks desired angular rates. 
The sensitivity analysis is performed by individually scaling P- and D-gains and analyzing the tracking performance. 
The analysis is performed on the \textit{RaceA} maneuver in the nominal simulation setting. 
For reference, the sensitivity analysis is performed also for the MPC-CTBR baseline.\\
Figure~\ref{fig:llc_ablation} shows the results of this sensitivity analysis. 
Starting from the nominal PD-tuning with a scaling factor of (1.0, 1.0), 121 controller tunings have been tested with scaling factors in the range [0.0, 100.0]. 
The learned CTBR policies show comparable robustness against changes in the low-level controller as the MPC-CTBR baseline. 
\begin{figure}
    \centering
    \includegraphics[width=0.49\linewidth]{figures/llc_ablation/llc_ablation_ctbr.eps}
    \includegraphics[width=0.49\linewidth]{figures/llc_ablation/llc_ablation_mpc.eps}
    \caption{\rev{Positional tracking error in meters for varying low-level controllers on \textit{RaceA} for the MPC-CTBR baseline (left) and the learned CTBR policies (right). The low-level PD controller is randomized by individually scaling its P- and D-gains. Tracking errors are clipped at 5m. The learned CTBR policies exhibit a significant robustness against changes in the underlying low-level controller that is comparable to the MPC-CTBR baseline.}}
    \label{fig:llc_ablation}
\end{figure}
}

\rev{
\mypara{Influence of Observation History}
We investigate the impact of the history length $H$ on the tracking performance of our trained policies. 
All policies are trained using domain randomization and only differ in the length of the history of prior states and actions observed. We train policies for $H=\lbrace1, 5, 10\rbrace$. The reference length $R=10$ is kept constant.\\
The results of this ablation study are shown in Table~\ref{tab:history_ablation}. 
Policies with access to a history of observations strictly outperform reactive policies for all control input modalities on all tested trajectories.
Transitioning from no history (H1) to a medium-sized history (H5) leads to a larger improvement in performance compared to the difference between a long history (H10) and a medium-sized history (H5). 
Policies operating at a lower abstraction level (SRT, CTBR) show a larger sensitivity to history length than policies operating at a higher abstraction level (LV). 
}

\begin{table}[h]
\caption{\textnormal{\rev{Ablation of the impact of the history length $H$ on the tracking performance, evaluated in a quadrotor simulator based on blade-element momentum theory. Results report mean and standard deviation for 10 trained policies.}}}
\label{tab:history_ablation}
\vspace*{3pt}
\small
\setlength{\tabcolsep}{2pt}
\begin{tabularx}{1\linewidth}{X|cccccccc}
 & Hover & RandA & RandB & RandC & RaceA & RaceB & Split-S & RaceC \\
\midrule
SRT-H1      & crash &  crash  & crash & crash & crash & crash & crash & crash\\
CTBR-H1      &1.7$\pm$0.5 & 5.4$\pm$2.9 & 5.0$\pm$1.2 & 6.2$\pm$1.4 & 16.4$\pm$3.0 & 46.5$\pm$18.6 & 12.3$\pm$3.6 & 67.0$\pm$16.0 \\
LV-H1     & 7.6$\pm$2.0 & 21.5$\pm$6.7 & 79.2$\pm$7.6 & 133$\pm$30 & 168$\pm$55 & 217$\pm$19 & 138$\pm$48 & 210$\pm$35 \\
\midrule
SRT-H5      & 0.106 &  crash &  crash &  crash & crash & crash & crash & crash\\
CTBR-H5     & 1.2$\pm$0.4 & 2.3$\pm$0.9 & 4.4$\pm$1.7 & 4.0$\pm$1.5 & 7.7$\pm$2.9 & 11.5$\pm$4.2 & 7.7$\pm$3.2 & 28.5$\pm$17.6 \\
LV-H5      &7.2$\pm$0.9 & 19.2$\pm$1.7 & 67.7$\pm$9.0 & 98.3$\pm$24.6 & 155.3$\pm$9.8 & 182.0$\pm$24.9 & 103.3$\pm$24.6 & 196.0$\pm$10.7 \\
\midrule
SRT-H10      & 11.3$\pm$4.5 &  12.0$\pm$4.0 &  14.4$\pm$2.4 &  17.6$\pm$5.9 & crash & crash & crash & crash\\
CTBR-H10     & 0.6$\pm$0.5 & 1.2$\pm$0.5 & 2.2$\pm$0.8 & 2.6$\pm$0.8 & 5.6$\pm$1.7 & 10.0$\pm$4.0 & 6.9$\pm$2.6 & 14.9$\pm$5.5 \\
LV-H10      &6.7$\pm$2.0 & 17.8$\pm$1.4 & 57.0$\pm$12.0 & 78.9$\pm$13.4 & 144.0$\pm$20.1 & 161.4$\pm$17.0 & 83.8$\pm$9.7 & 161.7$\pm$22.0
\end{tabularx}

\end{table}

\rev{
\mypara{Influence of Reference Length}
We investigate the impact of the reference length $R$ on the tracking performance of our trained policies. 
All policies are trained using domain randomization and only differ in the length of the receding-horizon reference. We train policies for $R=\lbrace1, 5, 10\rbrace$. The history length $H=10$ is kept constant.\\
The results of this ablation study are shown in Table~\ref{tab:reference_ablation}. 
Policies with a longer reference length of $R=10$ perform superior compared to policies with only access to a single reference $R=1$ or a short reference $R=5$. 
This trend is consistent across action spaces and is more pronounced for more aggressive maneuvers.
}

\begin{table}[h]
\caption{\textnormal{\rev{Ablation of the impact of the reference length $R$ on the tracking performance, evaluated in a quadrotor simulator based on blade-element momentum theory. Results report mean and standard deviation for 10 trained policies.}}}
\label{tab:reference_ablation}
\vspace*{3pt}
\small
\setlength{\tabcolsep}{2pt}
\begin{tabularx}{1\linewidth}{X|cccccccc}
 & Hover & RandA & RandB & RandC & RaceA & RaceB & Split-S & RaceC \\
\midrule
SRT-R1      & 14.0$\pm$2.4 & 17.7$\pm$2.1  & crash & crash & crash & crash & crash & crash\\
CTBR-R1      &5.6$\pm$2.1 & 7.3$\pm$2.4 & 7.6$\pm$2.0 & 6.1$\pm$2.4 & 11.8$\pm$5.7 & 33.0$\pm$8.1 & 22.1$\pm$6.4 & 43.3$\pm$14.6\\
LV-R1     & 10.6$\pm$3.4 & 27.9$\pm$9.4 & 73.3$\pm$13.5 & 101$\pm$17 & 174$\pm$22 & 191$\pm$21 & 97.9$\pm$10.6 & 218$\pm$41 \\
\midrule
SRT-R5      & 12.3$\pm$2.4 & 15.0$\pm$2.9 &  crash &  crash & crash & crash & crash & crash\\
CTBR-R5     & 0.9$\pm$0.2 & 1.6$\pm$0.3 & 4.5$\pm$1.7 & 5.0$\pm$2.4 & 10.1$\pm$5.2 & 18.0$\pm$7.0 & 11.7$\pm$5.3 & 23.4$\pm$6.0 \\
LV-R5      &7.8$\pm$1.6 & 20.3$\pm$3.6 & 62.3$\pm$7.5 & 87.7$\pm$12.4 & 162.0$\pm$25.5 & 178.3$\pm$23.9 & 92.3$\pm$12.1 & 188.9$\pm$38.5\\
\midrule
SRT-R10      & 11.3$\pm$4.5 &  12.0$\pm$4.0 &  14.4$\pm$2.4 &  17.6$\pm$5.9 & crash & crash & crash & crash\\
CTBR-R10     & 0.6$\pm$0.5 & 1.2$\pm$0.5 & 2.2$\pm$0.8 & 2.6$\pm$0.8 & 5.6$\pm$1.7 & 10.0$\pm$4.0 & 6.9$\pm$2.6 & 14.9$\pm$5.5 \\
LV-R10      &6.7$\pm$2.0 & 17.8$\pm$1.4 & 57.0$\pm$12.0 & 78.9$\pm$13.4 & 144.0$\pm$20.1 & 161.4$\pm$17.0 & 83.8$\pm$9.7 & 161.7$\pm$22.0
\end{tabularx}

\end{table}

\subsection{Tracking Performance}
\rev{
In addition to the tracking errors reported in Section~\ref{sec: exp}, we provide trajectory plots for the test trajectory \textit{RaceA}. 
We show plots for both simulation settings evaluated in the experimental section: the nominal simulation and the simulation based on blade-element momentum theory with 20ms delay.
Each plot illustrates the reference position and the actual position of the platform. 
In case of a crash, the rollout is terminated (Figure~\ref{fig:tracking_performance_srt_bem}).
}

\rev{
\mypara{Nominal Model}
Figures~\ref{fig:tracking_performance_srt_nom}, \ref{fig:tracking_performance_ctbr_nom}, \ref{fig:tracking_performance_lv_nom} illustrate the positional tracking performance of each policy type on the maneuver \textit{RaceA} in the nominal simulation setting.
The corresponding numerical tracking errors can be found in Table~\ref{tab:pos_tracking_vanilla}.
While SRT (Figure~\ref{fig:tracking_performance_srt_nom}) and CTBR (Figure~\ref{fig:tracking_performance_ctbr_nom}) achieve near-perfect performance, LV (Figure~\ref{fig:tracking_performance_lv_nom}) exhibits significant tracking error, especially in high-acceleration regimes of the trajectory.
}

\rev{
\mypara{Model Mismatch}
Figures~\ref{fig:tracking_performance_srt_bem}, \ref{fig:tracking_performance_ctbr_bem}, \ref{fig:tracking_performance_lv_bem} illustrate the performance of each policy type on the maneuver \textit{RaceA} in the model mismatch setting, which uses blade-element momentum theory to model the aerodynamic forces and torques acting on the platform.
The corresponding numerical tracking errors can be found in Table~\ref{tab:pos_tracking_bem_20_latency}.
SRT policies are very sensitive to changes in the quadrotor model, leading to a crash already after 5.5s as shown in Figure~\ref{fig:tracking_performance_srt_bem}. 
In contrast, CTBR policies manage to complete the entire trajectory with similar performance as in the nominal setting (Figure~\ref{fig:tracking_performance_ctbr_bem}).
LV policies are also robust to changes in platform dynamics, with tracking performance comparable to the nominal case. 
Also in the model mismatch setting, LV policies show large tracking errors, especially in high-acceleration regimes of the trajectory (Figure~\ref{fig:tracking_performance_lv_bem}).
}

\begin{figure}[h]
    \centering
    \input{figures/tracking_performance/srt_000_eval_04_cpc165_extended.csv}
    \vspace{-0.25cm}
    \caption{Tracking performance of SRT on test trajectory RaceA evaluated with the nominal quadrotor model.}
    \label{fig:tracking_performance_srt_nom}
    \input{figures/tracking_performance/ctbr_000_eval_04_cpc165_extended.csv}
    \vspace{-0.25cm}
    \caption{Tracking performance of CTBR on test trajectory RaceA evaluated with the nominal quadrotor model.}
    \label{fig:tracking_performance_ctbr_nom}
    \input{figures/tracking_performance/linvel_000_eval_04_cpc165_extended.csv}
    \vspace{-0.25cm}
    \caption{Tracking performance of LV on test trajectory RaceA evaluated with the nominal quadrotor model.}
    \label{fig:tracking_performance_lv_nom}
\end{figure}

\begin{figure}[h]
    \centering
    \input{figures/tracking_performance/bem_srt_000_eval_04_cpc165_extended.csv}
    \vspace{-0.25cm}
    \caption{Tracking performance of SRT on test trajectory RaceA evaluated in the BEM simulation.}
    \label{fig:tracking_performance_srt_bem}
    \input{figures/tracking_performance/bem_ctbr_000_eval_04_cpc165_extended.csv}
    \vspace{-0.25cm}
    \caption{Tracking performance of CTBR on trajectory RaceA evaluated in the BEM simulation.}
    \label{fig:tracking_performance_ctbr_bem}
    \input{figures/tracking_performance/bem_linvel_000_eval_04_cpc165_extended.csv}
    \vspace{-0.25cm}
    \caption{Tracking performance of LV on test trajectory RaceA evaluated in the BEM simulation.}
    \label{fig:tracking_performance_lv_bem}
\end{figure}

\subsection{Reference Trajectories}
The control policies are trained on a set of feasible reference trajectories. 
We generate smooth trajectories in position using two approaches: (i)~we generate random circular trajectories of different inclination angles, radii, and speeds; (ii)~we generate random position trajectories by combining periodic exponential-sine-squared kernels of different magnitudes and frequencies. 
Both type of trajectories are extended to full-state quadrotor trajectories by exploiting the differential flatness property of the quadrotor dynamics~\cite{Faessler18ral}.
In total we generate over 600 trajectories covering speeds from \SI{0}{\meter\per\second} up to \SI{20}{\meter\per\second} and accelerations up to \SI{35}{\meter\per\second\squared}.
\rev{An illustration of one sample of both trajectory types is provided in Figure~\ref{fig:reference_trajectory_symbolic} and Figure~\ref{fig:reference_trajectory_random}.}
\begin{figure}[h]
    \centering
    \input{figures/symbolic}
    \caption{Illustration of a sample circular reference trajectory in the training set. Circular trajectories are generated with random inclination angles, radii and speeds.}
    \label{fig:reference_trajectory_symbolic}
    \input{figures/random}
    \caption{Illustration of a sample random reference trajectory in the training set. Random trajectories are generated by combining periodic exponential-sine-squared kernels of different magnitudes and frequencies, resulting in a smooth position trajectory. Reference attitude and angular rate is then computed using the differential flatness property of the quadrotor platform.}
    \label{fig:reference_trajectory_random}
\end{figure}
